# Supplementary material for: Theory of Andreev Blockade in a Double Quantum Dot with a Superconducting Lead
Source: arXiv:1810.05112 ancillary file (2021-06-14)
Supplement: Supplementary file 1 [file supplement.pdf]

# Supplemental Information: Andreev Blockade in a Double Quantum Dot with a Superconducting Lead

David Pekker and Sergey M. Frolov
*Department of Physics and Astronomy, University of Pittsburgh, Pittsburgh, PA, 15260*

This supplement is composed of two sections: in section "Transport formalism" we provide the details of our transport calculations that were omitted from the main text for clarity; in section "Additional data" we provide supporting plots.

## I. TRANSPORT FORMALISM

In this section of the supplement we provide the details of the transport formalism that we use in the main paper. We begin by constructing a minimal quantum Hamiltonian of the double quantum dot system coupled to normal and superconducting leads. With the exception of Andreev reflection, all other electron tunneling processes are treated as incoherent processes that drive transitions between the eigenstates of the quantum Hamiltonian. We describe the resulting population dynamics, and consequent transport properties, using the classical master equation formalism.

### A. Minimal quantum Hamiltonian of the double quantum dot system with Andreev reflection

To construct the quantum dot Hamiltonian in the presence of Andreev reflection, we supplement the quantum dot charging Hamiltonian with the Andreev Hamiltonian

$$H = H_{\text{QD}} + H_{\text{Andreev}}. \tag{1}$$

The quantum dot charging Hamiltonian is

$$H_{\text{QD}} = \sum_{i,\sigma} \epsilon_{i,\sigma} n_{i,\sigma} + \sum_{i=\{1,2\}} U_i n_{i,\uparrow} n_{i,\downarrow} + U_{12}(n_{1,\uparrow}+n_{1,\downarrow})(n_{2,\uparrow}+n_{2,\downarrow}), \tag{2}$$

where $n_{i,\sigma}$ is the number operator for electron with spin $\sigma \in \{\uparrow,\downarrow\}$ on quantum dot $i \in \{1,2\}$; the first term describes the single-particle energy that is tuned by the gate voltage $\epsilon_{i,\sigma} = V_{gi}$; the second term describes the quantum dot self-capacitance energy $U_i$; and the final term describes the quantum dot cross-capacitance energy $U_{12}$.

The Andreev Hamiltonian, which describes the tunneling of Cooper pairs between the quantum dot and the adjacent superconducting lead, is

$$H_{\text{Andreev}} = \sum_{i\in\text{SC}} \left[\left(\Delta_i c^\dagger_{\uparrow,i} c^\dagger_{\downarrow,i} + \text{h.c.}\right) + 2eV_i n_{i,\uparrow} n_{i,\downarrow}\right], \tag{3}$$

where the sum runs over the quantum dots that are adjacent to superconducting leads. For the N-QD-QD-N device $H_{\text{Andreev}}$ is omitted, for N-QD-QD-SC device the sum runs over $i = \{2\}$, and for SC-QD-QD-SC device the sum runs over $i = \{1,2\}$. The first term of $H_{\text{Andreev}}$ describes the Andreev reflection process. The second term corresponds to the electrochemical potential of a Cooper pair in the $i$-th lead (biased to voltage $V_i$) and describes the change in the energy of the superconducting lead when a Cooper pair hops onto the quantum dot. The Andreev Hamiltonian is the minimal modification to $H_{\text{QD}}$ needed to describe the loop-like features that are commonly observed in transport through quantum dots coupled to superconducting leads [1, 2].

We note that our minimal quantum Hamiltonian has no inter-dot electron tunneling nor single-electron tunneling between the quantum dots and the leads. Consequently the eigenstates of the quantum Hamiltonian are product states over the quantum dots.

### B. Eigenstates of the minimal quantum Hamiltonian

The eigenstates of quantum dots adjacent to normal metal leads are just the charging states: $|0\rangle$, $|\uparrow\rangle$, $|\downarrow\rangle$, and $|\uparrow\downarrow\rangle$. On the other hand, for quantum dots adjacent to superconducting leads the empty and double occupied states are mixed by Andreev reflection resulting in the following set of eigenstates:

- Odd parity state $|\uparrow\rangle$
- Odd parity state $|\downarrow\rangle$
- Even parity state $|+\rangle = \sin(\theta)|0\rangle + \cos(\theta)|\uparrow\downarrow\rangle$
- Even parity state $|-\rangle = \cos(\theta)|0\rangle - \sin(\theta)|\uparrow\downarrow\rangle$

where the angle $\theta$ depends on the parameters that go into $H$. We shall assume that $\theta$ is chosen so that the $|+\rangle$ even parity state has lower energy than the $|-\rangle$ state. Further, henceforth we will truncate the basis for quantum dots adjacent to superconducting leads to the state $|\uparrow\rangle$, $|\downarrow\rangle$, and $|\text{even}\rangle = |+\rangle$.

The eigenstates of the N-QD-QD-SC device that we consider in the main text are $\{|0\rangle, |\uparrow\rangle, |\downarrow\rangle, |\uparrow\downarrow\rangle\} \bigotimes \{|\uparrow\rangle, |\downarrow\rangle, |\text{even}\rangle\}$, where the notation $\{\dots\}$ means that we have to choose one element of the set in the curly braces.

### C. Transition rates: rules for adding/removing electrons to quantum dots adjacent to superconducting leads

Having determined the eigenstates of $H$, we can work out the rules for adding and removing single electrons from the quantum dot. The essential feature we must take care of in constructing these rules is that the addition (or removal) of electrons to the dot can lead to transitions between states with different number of Cooper pairs in the superconducting lead(s). To keep track of the number of electrons in the superconducting lead we use the notation $|N_{\text{lead}}, QD\rangle$ where $N_{\text{lead}}$ counts the number of electrons in the superconducting lead and $|QD\rangle$ is the state of the adjacent quantum dot.

For example, consider the case in which the quantum dot is gated so that the ground state has even parity. In this case the matrix element for adding an electron to the quantum dot is:

$$\langle N, \uparrow | c_\uparrow^\dagger \left[\cos(\theta)|N, 0\rangle + \sin(\theta)|N-2, \uparrow\downarrow\rangle\right], \quad (4)$$

where $c_\uparrow^\dagger$ is the up-spin electron creation operator on the quantum dot. We observe that both the initial and the final states are in the same Cooper pair number block of $H_{\text{SC/QD}}$. Hence, the energy of the electron being added to the quantum dot is $E_{\text{add}} = E_{\text{x}} - E_{\text{gs}}$, i.e. the difference between the energies of the odd parity excited state and of the even parity ground state. Note that if the electron is being added via an inelastic process, then $E_{\text{add}} > E_{\text{x}} - E_{\text{gs}}$. On the other hand, if we would like to remove an electron from the quantum dot, the appropriate matrix element is

$$\langle N-2, \downarrow | c_\uparrow \left[\cos(\theta)|N, 0\rangle + \sin(\theta)|N-2, \uparrow\downarrow\rangle\right]. \quad (5)$$

In this case the final state is in a different $H_{\text{SC/QD}}$ block as compared to the initial state. Hence the energy of the removed electron is $E_{\text{rm}} = E_{\text{gs}} - E_{\text{x}} + 2eV$ (or $E_{\text{rm}} < E_{\text{gs}} - E_{\text{x}} + 2eV$ for an inelastic process).

The particle-hole picture is a convenient way to track these energies. Introducing the energy $\delta = E_{\text{x}} - E_{\text{gs}} - eV$, the energy to add an electron becomes $eV + \delta$ (i.e. a filled single-particle state of energy at least $eV + \delta$ can give up its electron to the quantum dot). The energy to remove an electron becomes at most $eV - \delta$ (i.e. an empty single-particle state of energy at most $eV - \delta$ can accept the electron). The full set of rules for adding and removing electrons is summarized in Fig. 1.

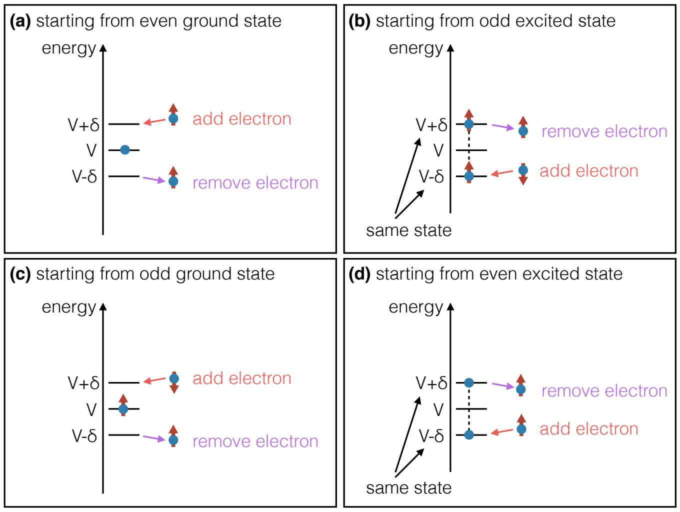


FIG. 1. Rules for adding and removing electrons from a quantum dot Andreev coupled to a superconducting lead. The lead is biased to voltage $V$, and the singlet double splitting on the quantum dot is $\delta$. Initial states with no arrows [panels (a) and (d)] are even parity states, while initial states with arrows [panels (b) and (c)] are odd parity states. States connected by a dotted lines [panels (b) and (d)] correspond to the same state with a different number of Cooper pairs in the superconducting lead. The levels on the right correspond to single electron levels that will be resonantly coupled to the quantum dot for electron addition/removal, as labeled.

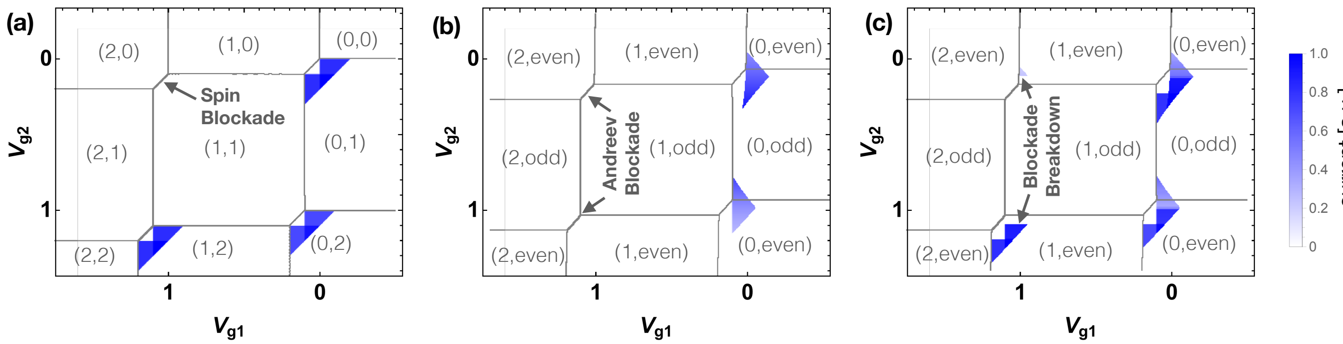


FIG. 2. Same as Fig. 2 of the main paper with reversed source-drain bias.

### D. Master equation

The inputs into the master equation formalism are the eigenstates of the double dot subsystem along with rates for elastic processes that move electrons between the leads and the quantum dots along with inelastic rates for moving electrons between the quantum dots.

Having obtained the set of eigenstates $\psi_\alpha$ and eigenenergies $E_\alpha$ of the double quantum dot system we can write down the conventional classical master equation for the populations $P_\alpha$.

$$\partial_t P_\alpha = -\sum_{\alpha\neq\beta} \Gamma_{\alpha\to\beta} P_\alpha + \sum_{\beta\neq\alpha} \Gamma_{\beta\to\alpha} P_\beta. \tag{6}$$

The only modification needed to the conventional formalism described in Ref. [3] is to account for processes in which the number of Cooper pairs changes in the superconducting lead. These modifications are described in the previous subsection "Transition rates: rules for adding/removing electrons to quantum dots adjacent to superconducting leads."

We assume that electron tunneling between the quantum dots is an inelastic process. At zero temperature this process can take place whenever the initial state is higher in energy than the final state. At finite temperature we use the following functional form for the rate: $\Gamma(\Delta E) = \Gamma_{12}\left[1 + \tanh(\Delta E/2T)\right]/2$, where $\Delta E$ is the energy difference between the initial and final state and $\Gamma_{12}$ is the rate constant.

When computing the current through the device, we use the current operator between the two quantum dots. We specifically avoid using the current operator between a quantum dot and the adjacent lead in order to escape the complication of having to account for the Cooper pair number if the lead is superconducting.

## II. ADDITIONAL DATA

### A. Andreev blockade when source drain bias is reversed

In Fig. 2 of this supplement we re-plot Fig. 2 of the main text with the source drain bias reversed. Comparing these two figures we observe that upon flipping the bias: The Pauli blockade shifts to the $(1,1) \to (2,0)$ charge degeneracy point and the direction of the triangles flips [panel (a)]. The Andreev blockade shifts to the two $(1,\text{odd}) \to (2,\text{even})$ charge degeneracy points and the direction of the triangles flips [panel (b)].


[1] E. J. Lee, X. Jiang, M. Houzet, R. Aguado, C. M. Lieber, and S. De Franceschi, Nature nanotechnology **9**, 79 (2014).

[2] Z. Su, A. B. Tacla, M. Hocevar, D. Car, S. R. Plissard, E. P. A. M. Bakkers, A. J. Daley, D. Pekker, and S. M. Frolov, Nature Communications **8**, 585 (2017).

[3] C. W. J. Beenakker, Phys. Rev. B **44**, 1646 (1991).
